# Supplementary material for: WaveStitch: Flexible and Fast Conditional Time Series Generation with Diffusion Models
Source: arXiv:2503.06231 source file (2025-11-04)
Supplement: Supplementary file 1 [file appendix.tex]

% \documentclass[sigconf,nonacm, colorlinks]{acmart}
% \acmSubmissionID{280}

% \setcopyright{acmlicensed}
% \copyrightyear{2018}
% \acmYear{2018}
% \acmDOI{XXXXXXX.XXXXXXX}
% %% These commands are for a PROCEEDINGS abstract or paper.
% \acmConference[Conference acronym 'XX]{Make sure to enter the correct
%   conference title from your rights confirmation email}{June 03--05,
%   2018}{Woodstock, NY}

% \usepackage{amsmath,amsfonts}
% \usepackage{algorithm}
% \usepackage[noend]{algpseudocode}
% \usepackage{graphicx}
% \usepackage{subcaption}
% \usepackage{textcomp}
% \usepackage[most]{tcolorbox}
% \usepackage{xcolor}
% \usepackage[table]{xcolor}
% \usepackage{makecell}
% % \usepackage{xcolor}
% \usepackage{booktabs}
% \usepackage{xspace}
% \usepackage{pifont}
% \usepackage{booktabs}
% \usepackage{graphicx}
% \usepackage{multirow}
% \usepackage{hyperref}

%            % color for citations           % color for URLs

% \definecolor{mygray}{gray}{0.95}
% \newcommand{\bemph}[1]{\textbf{\textit{#1}}}
          
% \newcommand{\algo}{\texttt{WaveStitch}\xspace}
% \newcommand{\algoar}{\texttt{WaveStitchAR}\xspace}

% \begin{document}
% \title{\algo: Flexible and Fast Conditional Time Series Generation With Diffusion Models (Appendix)}

% \maketitle

\section*{A. RePaint-based WaveStitch}
To condition on both metadata and available signal values during inference, we implement a RePainting-based version of \algo, detailed in \hyperref[alg:synthrp]{Algorithm 3}. First, we apply a conditional mask to identify the known signal values, which is used to generate noised versions of the signal (step 1, \autoref{fig:repaintingrp}). The denoising process is then applied to the entire signal, with conditions re-introduced at each iteration to adjust the unconstrained parts of the signal in alignment with the known values.

We parallelize the generation of time series segments using overlapping windows. Each mini-batch of windows is denoised in parallel, conditioned on the historical signals and metadata. To enforce \Description{A plot showing conditional denoising with observed values highlighted in orange.}coherence across windows, the RePaint-based stitching mechanism simply \textbf{overwrites} overlapping regions in each window with the corresponding region from the preceding window, gradually aligning non-overlapping parts in subsequent iterations (see \autoref{fig:stitchrp}, line \ref{ln:stitchrp}). This approach, ensures that coherence emerges progressively through iterative refinement. 

\section*{B. Impact of Guidance Strength (TSDiff)}
 For transparency on the tuning sensitivity of baselines, we included results analyzing the impact of guidance strength on \texttt{TSDiff} performance in \autoref{tab:tsdiffres} below, to contextualize performance variations. As seen in the table, the guidance strength of 0.5 gives the best performance on average, which we have consistently used for the experiments in the main text as well.
 \begin{algorithm}[tb]
\caption{WaveStitch Inference with RePainting}
\label{alg:synthrp}
\begin{algorithmic}[1]

\State \textbf{Input:} 
Windowed metadata ($\mathcal{A}_w$), masks ($\mathcal{M}_w$), and signals ($\mathcal{X}_w$); Timesteps $M$, window size \( w \); Stride \( s \); mini-batch size \(b\); diffusion parameters \( \{ \alpha_t, \beta_t, \overline{\alpha}_t\} \); metadata \( \mathcal{A} = \{\mathbf{a}^{(i)}\}_{i=1}^M \); Denoiser \( f_\theta \).

% \State \textbf{Create windowed samples:}
% \label{ln:windowingrp}
% \vspace{-5pt}
% \[
% \mathcal{X}_w = \{ \mathbf{x}_w^{(i)} = \mathbf{x}^{(i.s - s + 1:i.s -s + w)} \}_{i=1}^{\left\lfloor {(M - w)}/{s} \right\rfloor}, 
% \]
% \[
% \mathcal{A}_w = \{ \mathbf{a}_w^{(i)} = \mathbf{a}^{(i.s - s + 1:i.s -s + w)} \}_{i=1}^{\left\lfloor {(M - w)}/{s} \right\rfloor}, 
% \]
% \[
% \mathcal{M}_w = \{ \mathbf{m}_w^{(i)} = \mathbf{m}^{(i.s - s + 1:i.s -s + w)} \}_{i=1}^{\left\lfloor {(M - w)}/{s} \right\rfloor}, 
% \]

\State \textbf{Initialize outputs:}
\vspace{-5pt}
\[
\mathcal{\hat{X}}_w = \{ \mathbf{\hat{x}}_{w,T}^{(j)}\sim \mathcal{N}(0,I) \}_{j=1}^{\left\lfloor {(M - w)}/{s} \right\rfloor} 
\] 
\vspace{-13pt}
\State \textbf{Divide $\mathcal{X}_w, \mathcal{A}_w, \mathcal{M}_w$ into $(M-w)/(b\times s)$ mini-batches}
% \State \textbf{Initialize output windows:}
% \vspace{-5pt}
% \[
% \mathcal{\hat{X}}_w = \{ \mathbf{\hat{x}}_w^{(i)} = (1-\mathbf{m}_w^{(i)})\cdot \mathbf{x}_w^{(i)} + \mathbf{m}_w^{(i)}\cdot \mathbf{z}^{(i)} \}_{i=1}^{\left\lfloor {(M - w)}/{s} \right\rfloor} 
% \], where \(\mathbf{z}^{(i)}\sim \mathcal{N}(0,I_{w\times C})\)

% \State \textbf{Divide $\mathcal{X}_w, \mathcal{A}_w, \mathcal{M}_w$ into $(M-w)/(b\times s)$ mini-batches}

\For{each mini-batch}
  \For{(\(\mathbf{x}_w^{(j)}, \mathbf{a}_w^{(j)}, \mathbf{m}_w^{(j)}\)) in mini-batch in \textbf{parallel}:}
    \For{step \( t = T, T-1, \dots, 1 \)}
      \State \textbf{Conditional Forward noising}: 
        \label{ln:condfwdnoisingrp}
            \[
            \mathbf{\hat{x}}_{w,t}^{(i)} = (1-\mathbf{m}_w^{(i)})\cdot (\sqrt{\overline{\alpha}_t} \cdot \mathbf{{x}}_w^{(i)} + \sqrt{1 - \overline{\alpha}_t} \cdot \epsilon^{(i)}) + \mathbf{m}_w^{(i)} \cdot \mathbf{\hat{x}}_{w,t}^{(i)}\]
        \vspace{-15pt}
        \State \textbf{One-step denoising}:
        \label{alg:denoisingrp}
        \vspace{-5pt}
        \[
        \mathbf{\hat{x}}_{w,t-1}^{(i)} = \frac{1}{\sqrt{\alpha_t}} \left( \mathbf{\hat{x}}_{w,t}^{(i)} - \frac{1 - \alpha_t}{\sqrt{1 - \overline{\alpha}_t}} \cdot f_{\theta} \left( \mathbf{a}_w^{(i)}, \mathbf{\hat{x}}_{w,t}^{(i)},t \right) \right)
        \]
        \vspace{-10pt}
        \State \textbf{Re-introduce conditions:}
        \[
        \mathbf{\hat{x}}_{w,t-1}^{(i)} = (1-\mathbf{m}_w^{(i)})\cdot \mathbf{x}_w^{(i)}
         + \mathbf{m}_w^{(i)}\cdot \mathbf{\hat{x}}_{w, t-1}^{(i)}\]
      \EndFor
      \If{\(s<w\)}
      \For{\(i > 1\) in \textbf{parallel}}
        \State \textbf{Stitch overlaps:}
    \label{ln:stitchrp}
    \vspace{-5pt}
    \[
    \mathbf{\hat{x}}_w^{(i)(1:w-s)} = \mathbf{\hat{x}}_w^{(i-1)(1+s:w)}
    \]
    \vspace{-15pt}
    \EndFor
    \EndIf
  \EndFor
\EndFor

\State \textbf{Merge windows:}
\vspace{-5pt}
\[
\mathcal{\hat{X}} = \mathbf{\hat{x}}_w^{(1)} \cup 
\left(
\bigcup_{i\geq 2} \mathbf{\hat{x}}_w^{(i)(w-s+1:w)}
\right)
\]
\vspace{-10pt}
\State \Return {\(\mathcal{\hat{X}}\)}

\end{algorithmic}
\end{algorithm}

 \begin{figure}[htb]
    \centering\includegraphics[width=0.40\textwidth]{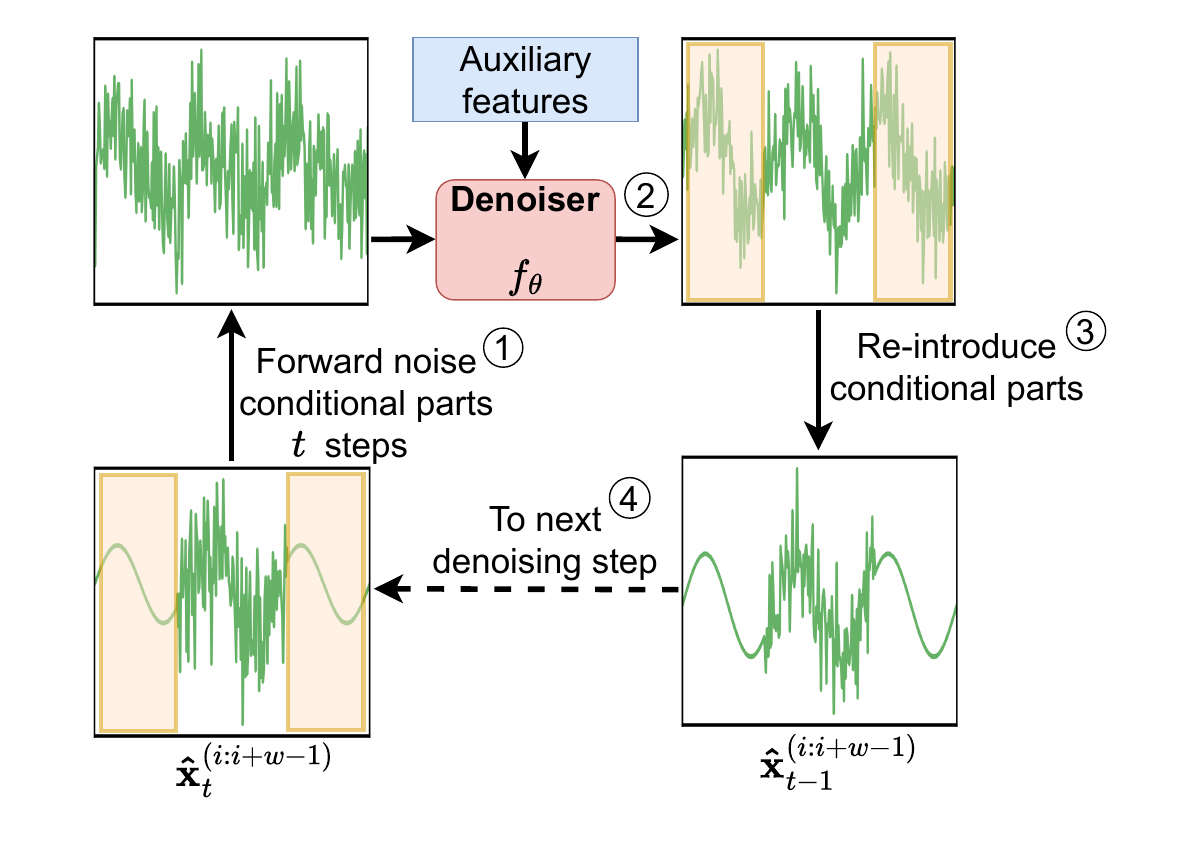}
    \caption{Conditional Denoising. Observed values in orange.}
    \Description{A plot showing conditional denoising with observed values highlighted in orange.}\label{fig:repaintingrp}
\end{figure}
\begin{figure}[htb]
    \centering\includegraphics[width=0.40\textwidth]{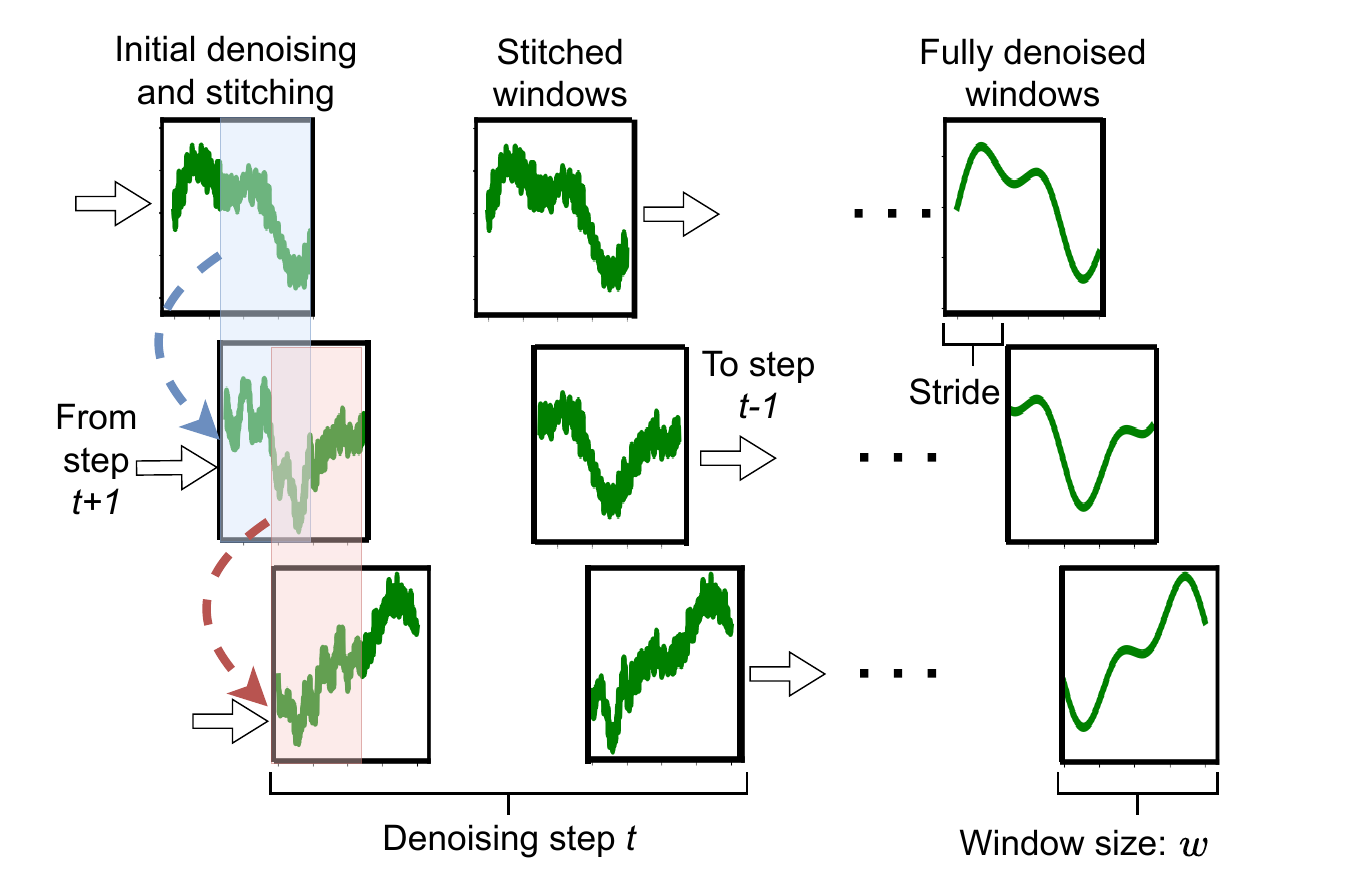}
    \caption{Parallel Denoising with Overlap Stitching}
    \label{fig:stitchrp}
\end{figure}
\begin{table}[htb]
\centering
\caption{\centering{{Comparison of performance (MSE$\downarrow$) of TSDiff under varying guidance strengths, for different datasets and tasks (\textit{R}/\textit{I}/\textit{B}). Best score is in bold and second-best is \underline{underlined}.}}}
\label{tab:tsdiffres}
\setlength{\tabcolsep}{3pt} % Reduce column spacing
 % Adjust row spacing
\fontsize{12}{15}\selectfont % Set font size (12pt with 15pt line spacing)

\scalebox{0.61}{
\begin{tabular}{lcccccccc}
\Xhline{1.5pt}
\textbf{} & \textbf{0.0} & \textbf{0.5} & \textbf{1.0} & \textbf{2.0} \\
\midrule
\phantom{AT} (\bemph{R}) & $ 1.469_{.002}$ & $ 1.223_{.007}$ & $ \underline{1.174_{.002}}$ & $ \mathbf{1.062_{.022}}$ \\
AT (\bemph{I}) & $ 1.964_{.020}$ & $ \underline{1.480_{.003}}$ & $ \mathbf{1.395_{.020}}$ & $ 1.932_{.002}$ \\
\phantom{AT} (\bemph{B}) & $ \mathbf{1.331_{.012}}$ & $ 1.567_{.032}$ & $ \underline{1.446_{.007}}$ & $ 1.609_{.004}$ \\
\rowcolor{mygray}
\phantom{MT} (\bemph{R}) & $ 1.026_{.011}$ & $ \underline{0.964_{.009}}$ & $ \mathbf{0.880_{.014}}$ & $ 1.017_{.007}$ \\
\rowcolor{mygray}
MT (\bemph{I}) & $ \mathbf{0.573_{.036}}$ & $ \underline{0.768_{.027}}$ & $ 0.846_{.073}$ & $ 0.809_{.041}$ \\
\rowcolor{mygray}
\phantom{MT} (\bemph{B}) & $ \underline{0.215_{.008}}$ & $ \mathbf{0.200_{.010}}$ & $ 0.292_{.012}$ & $ 0.267_{.006}$ \\
\phantom{BQ} (\bemph{R}) & $ 2.333_{.014}$ & $ \mathbf{1.763_{.017}}$ & $ 2.444_{.010}$ & $ \underline{2.158_{.009}}$ \\
BQ (\bemph{I}) & $ \mathbf{1.342_{.011}}$ & $ \underline{1.422_{.025}}$ & $ 2.780_{.016}$ & $ 1.514_{.010}$ \\
\phantom{BQ} (\bemph{B}) & $ 0.244_{.022}$ & $ \mathbf{0.162_{.007}}$ & $ 0.167_{.007}$ & $ \underline{0.164_{.012}}$ \\
\rowcolor{mygray}
\phantom{RS} (\bemph{R}) & $ 0.785_{.008}$ & $ 0.893_{.021}$ & $ \mathbf{0.688_{.007}}$ & $ \underline{0.760_{.011}}$ \\
\rowcolor{mygray}
RS (\bemph{I}) & $ 0.971_{.037}$ & $ 0.827_{.032}$ & $ \underline{0.723_{.007}}$ & $ \mathbf{0.637_{.025}}$ \\
\rowcolor{mygray}
\phantom{RS} (\bemph{B}) & $ \underline{0.298_{.006}}$ & $ 0.458_{.011}$ & $ \mathbf{0.276_{.004}}$ & $ 0.394_{.007}$ \\
\phantom{PE} (\bemph{R}) & $ \mathbf{1.405_{.011}}$ & $ 1.667_{.005}$ & $ 2.105_{.003}$ & $ \underline{1.410_{.008}}$ \\
PE (\bemph{I}) & $ 2.171_{.092}$ & $ \mathbf{1.179_{.061}}$ & $ \underline{1.798_{.033}}$ & $ 2.538_{.039}$ \\
\phantom{PE} (\bemph{B}) & $ \mathbf{0.369_{.001}}$ & $ 0.469_{.002}$ & $ \underline{0.407_{.001}}$ & $ 0.469_{.001}$ \\
\midrule
Avg. & \underline{1.099} & \textbf{1.002} & 1.161 & 1.116\\
\Xhline{1.5pt}
\end{tabular}}
\end{table}

% \end{document}
